# Supplementary material for: Time-optimal control with direct collocation and variable discretization
Source: arXiv:2005.12136 source file (2020-05-25)
Supplement: Supplementary file 1 [file appendix.tex]

% !TeX spellcheck = en_US

\section{Complimentary Stability Results and Proofs} % TODO: name? weitere unterteilung in mehrere sections?
\label{app:extensions:uniform:stability}

A function $\fundef{\alpha}{\realposzero}{\realposzero}$ is of class~$\Kfun$ if it is continuous and strictly increasing with $\alpha(0)=0$.
If in addition $\alpha$ is unbounded, then it is of class $\Kinffun$.

\begin{defn}[Asymptotic Stability]
	\label{thm:lyapunov_asymp_stab}
	Let $\xf \in \xset$ be a steady state of system~\eqref{eq:closed_loop_system} and assume there exists a Lyapunov function $V$ on a forward invariant set $Y$ containing $\xf$ with the following properties:
	\begin{enumerate}%[label=(\roman*)]
		\item There exist functions $\alpha_1, \alpha_2 \in \Kinffun$ such that
		\begin{equation}
		\alpha_1 \big( \lVert \xmu - \xf \rVert \big) \leq V\big(\xmu\big) \leq \alpha_2 \big( \lVert \xmu - \xf \rVert \big)
		\label{app:eq:lyapunov_fun1}
		\end{equation}
		holds for all $\xmu \in Y$.
		\item There exists a function $\alpha_V \in \Kfun$ such that
		\begin{equation}
		\begin{split}
		V\Big( \xmusolfun\big(\tmud{n+1},\tmud{n}, \xmu(\tmud{n}) \big) \Big) \leq \\ V\big(\xmu(\tmud{n})\big) - \alpha_V \big( \lVert \xmu(\tmud{n}) - \xf \rVert \big)
		\end{split}
		\label{app:eq:lyapunov_fun2}
		\end{equation}
		holds for all $\xmu(\tmud{n}) \in Y$ with\\ $\xmusolfun\big(\tmud{n+1},\tmud{n}, \xmu(\tmud{n}) \big) \in Y$ and $n\in\naturalzero$. % TODO: check if we need to define tmud{n} and if n in \naturalzero is correct
	\end{enumerate}
	Then $\xf$ is asymptotically stable on $Y$.
\end{defn}

\begin{rem} \label{remark:uniformly_boundedness} % TODO: diesen remark vielleicht besser formulieren....
	Note, the previous definitions are defined for grid points $\tmud{n},$ with $n \in \naturalzero$ which is common for sampled-data systems in \MPC{}.
	This procedure is valid as long as $\xmuc{\tmu}$ is uniformly bounded, c.f.~\cite{gruene2017_book,nesic2004_tac}.
\end{rem}

The following lemmas provide intermediate results which are later required to verify Lyapunov function candidates.

\begin{lem}
	Let $\tfstar(\xs,N) \in \realpos$ denote the optimal transition time obtained from~\eqref{eq:ocp} with $\xs \in \rxset$,  $\xfset = \{ \xf \}$ and grid size $N\geq 1$.
	Further assume that the solution is feasible. % TODO: schöner formulieren?!
	Then, relation
	\begin{equation}
	\tfstar(\xs,N) > N\vardtmin \iff \xs \notin \Pfull{N}{N\vardtmin}
	\label{app:eq:vardt_not_in_p}
	\end{equation}
	holds for $\vardtmin \geq 0$.
	%The corresponding state trajectory $\xuc{t}$  obtained from either~\eqref{eq:uniform:fd:ocp}, \eqref{eq:uniform:ms:ocp} or~\eqref{eq:uniform:hs:ocp} with  $\xfset = \{ \xf \}$.
	%Further assume that \refassump{assum:uniform:optimal_solution} and \refassump{assump:ode_conditions} hold.
	\label{lemma:const_cost_dtstar_dtmin}
\end{lem}
\begin{IEEEproof}
	First, we abbreviate $\tfstar(\xs,N)$ with $\tfstar\mdef\tfstar(\xs,N)$, define $\tfmin\mdef N\vardtmin$ and consider the case $\xs \notin \Pfull{N}{\tfmin} \implies \tfstar > \tfmin$.
	The implication follows immediately from the definition of $\Pfull{N}{\tfmin}$ even for non-optimal $\tf$.
	By contraposition, the implication is equivalent to $\tfstar \leq \tfmin \implies \xs \in \Pfull{N}{\tfmin}$.
	The optimal solution is feasible by assumption and hence $\uadmset{\xs}{\tfstar} \neq \emptyset$ and $\tfstar \geq \tfmin$ are ensured such that condition $\tfstar \leq \tfmin$ is replaced by $\tfstar = \tfmin$.
	Consequently, all requirements for $\xs \in \Pfull{N}{\tfmin}$ are met. % TODO: ist das hier zu viel blabla?
	
	The second case $\tfstar > \tfmin \implies \xs \notin \Pfull{N}{\tfmin}$ does not hold for arbitrary (non-optimal) $\tf$ since control trajectories $u \in \uadmset{\xs}{\tf}$ could exists which start and end in $\Pfull{N}{\tfmin}$ but fulfill $\tfstar > \tfmin$ (for example keeping the system at the steady state).
	However, to show that the implication holds for $\tfstar$ subject to~\eqref{eq:ocp},
	consider the contraposition $\xs \in \Pfull{N}{\tfmin} \implies \tfstar \leq \tfmin$. 
	If $\xs \in \Pfull{N}{\tfmin}$ holds, then $\uadmset{\xs}{t}\neq \emptyset$ for $0 \leq t \leq \tfmin$ by \refdef{def:uniform:controllability_region}.
	Solving~\eqref{eq:ocp} results in minimum-time solutions adhering to constraint \mbox{$\tfmin \leq \tfstar$}
	and hence the only feasible transition time for $\xs \in \Pfull{N}{\tfmin}$ is $\tfstar=\tfmin$.
	The existence of this particular $u \in \mathscr{U}^N$ is confirmed by assumption (feasibility) even though it does not need to be unique.
	Consequently, $\tfstar=\tfmin$ proves the original implication $\xs \in \Pfull{N}{\tfmin} \implies$ \mbox{$\tfstar \leq \tfmin$}. 
	
	Finally, equivalence~\eqref{app:eq:vardt_not_in_p} follows immediately since both implications are true.
	%\qed	
	%since $\Pxf{N}$  all 
\end{IEEEproof}

\begin{lem} % TODO: üpberall x_mu(tmu) durch x_mu ersetzen??? brauchen wir das zeitargument???
	Let $\tfstar(\xs,N)$ denote the optimal time interval obtained from~\eqref{eq:ocp} with $\xs \in \rxset$, $\xf \in \rxset$, $\xfset = \{ \xf \}$ and grid size $N\geq 1$.
	Further assume that the solution is feasible. % TODO: schöner formulieren?! Und was ist mit Lipschitz hier? Das nehmen wir generell an
	Then, the optimal cost function value $\tfstar(\xs,N)$ is bounded by $\alpha_1, \alpha_2 \in \Kinffun$ such that
	\begin{equation}
	\alpha_1 \big( \lVert \xs - \xf \rVert \big) \leq \tfstar(\xs,N) \leq \alpha_2 \big( \lVert \xs - \xf \rVert \big)
	\label{eq:uniform:bounded_cost_function}
	\end{equation}
	% holds for all $\xs \in \rxset$ if $\vardtmin=0$ or $0 \leq \vardtmin < \vardtstar$ and $\xs \in \rxset \setminus \Pxf{N}$ otherwise.
	holds $\forall \xs \in \rxset$ if $\vardtmin=0$ or $\xs \in \rxset \setminus \Pfull{N}{N\vardtmin}$.
	\label{lemma:cost_lyapunov_bounds}
\end{lem}
\begin{IEEEproof}
	%It is to show that \eqref{eq:uniform:bounded_cost_function} holds for all $\xs \in \rxset\setminus \Pxf{N}$ and in case of $\vardtmin=0$ also for $\xs \in \rxset$.
	% The proof starts with $0 \leq \vardtmin < \vardtstar$.
	The proof starts with $\vardtmin = 0$ and we shorten $\tfstar(\xs,N)$ with $\tfstar\mdef\tfstar(\xs,N)$, $\tfmin \mdef N\vardtmin$ and $\uucstar{t,\xs,N}$ with $\uucstar{t}\mdef\uucstar{t,\xs,N}$. % TODO: with or by?
	By feasibility assumption, the optimal value $\tfstar\geq 0$ constitutes a unique minimizer and is finite for any finite $\xs$ and $\xf$.
	Furthermore, feasibility ensures that $\uadmset{\xs}{\tfstar}\neq \emptyset$ and the optimal control trajectory $\uucstar{t}$ is admissible. 
	% TODO: feasibility ensures that $\uadmset{\xs}{\tfstar}\neq \emptyset$ (könnte man auch allgemein in eine assumption packen).
	%	The proof shows the case $\vardtstar\geq\vardtmin=0$, since due to the exclusion according to $P_{N\vardtmin}(\xf)$  for any $\vardtmin>0$, the validity if \refassump{assum:uniform:optimal_solution} is met.
	The relation between $\xs$ and $\xf$ is given by~\eqref{eq:ivp:x}:
	\begin{equation}
	\xf = \xs + \int_{0}^{\tfstar} \f\big( \xc{t}, \uucstar{t} \big)\, \dt.
	\label{app:eq:bounded_cost:xs_xf_relation}
	\end{equation}
	The vector field $\f$ is Lipschitz in its first argument by assumption (see \refsec{sec:dyn_sys}) and $\uucstar{t} \in \ruset$ is bounded since $\ruset$ is compact by definition.
	Consequently, $\f$ is bounded on the close interval $[0, \tfstar]$ and there exists a scalar $C>0$ such that $\lVert \f\big(\x(t), \uucstar{t}\big) \rVert \leq C$ holds for $t\in [0, \tfstar]$.
	%For details on the relation between Lipschitz continuity and the boundedness of the function itself with respect to a bounded interval refer to~\cite{eriksson2004_book}.
	
	In order to proof the lower bound in~\eqref{eq:uniform:bounded_cost_function}, consider~\eqref{app:eq:bounded_cost:xs_xf_relation}, the triangle inequality in integral form and that $\f$ is Lipschitz:
%	\begin{equation}
%		\begin{split}
%		\lVert \xf - \xs \rVert &= \lVert \int_{0}^{\tfstar} \f\big(  \xc{t}, \uucstar{t} \big)\, \dt \rVert \\
%		&\leq \int_{0}^{\tfstar} \lVert \f\big(  \xc{t}, \uucstar{t} \big) \rVert\, \dt  \leq \int_{0}^{\tfstar} C\, \dt = C \tfstar.
%		\end{split}
%	\end{equation}
$\lVert \xf - \xs \rVert = \lVert \int_{0}^{\tfstar} \f\big(  \xc{t}, \uucstar{t} \big)\, \dt \rVert \\
\leq \int_{0}^{\tfstar} \lVert \f\big(  \xc{t}, \uucstar{t} \big) \rVert\, \dt  \leq \int_{0}^{\tfstar} C\, \dt = C \tfstar.$
	Since $C>0$, the lower bound is a $\Kinffun$ function and is given by $\tfstar \geq \lVert \xf - \xs \rVert/C = \alpha_1 \big( \lVert \xs - \xf \rVert \big).$
%	\begin{equation}
%	\tfstar \geq \frac{\lVert \xf - \xs \rVert}{C} = \alpha_1 \big( \lVert \xs - \xf \rVert \big).
%	\end{equation}
	It is possible to interpret the lower bound from a rather technical point of view. % TODO: das kann evtl weg
	Function $\f$ defines the velocity in the state space such that an upper bound $C$ represents the maximum velocity (w.r.t. the $\ell_2$-norm).
	So the minimum realizable transition time is estimated by the Euclidean distance $\lVert \xs - \xf \rVert$ divided by the maximum velocity~$C$.
	
	For the upper bound, consider that	
	$\lVert \xs - \xf \rVert = 0$ implies $\lVert \int_{0}^{\tfstar} \f\big(  \xc{t}, \uucstar{t} \big)\, \dt \rVert=0$.
	%	and hence either $N\vardtstar=0$ or $\f\big(  \xc{t}, \uucstar{t} \big)=0$. 
	% TODO: für den fall \vardtmin: können wir evtl auf das lemma mit der ruhelage zurückgreifen!!! um zu zeigen, dass assumption mit de roptimal solution
	% assum:uniform:optimal_solution wirklich auf f()=0 führt. Ansonsten ist offensichtlich N\vardt* = 0
	On the other hand, the norm of the integral must be strictly positive if $\lVert \xs - \xf \rVert > 0$.
	Note, the optimal control problem is feasible by assumption. % TODO: hier könnte man kürzen
	Consequently, there exists a scalar $\epsilon > 0$ such that
	$\lVert \xf - \xs \rVert = \lVert \int_{0}^{\tfstar} \f\big(  \xc{t}, \uucstar{t} \big)\, \dt \rVert \geq \epsilon$
%	\begin{equation}
%	\lVert \xf - \xs \rVert = \lVert \int_{0}^{\tfstar} \f\big(  \xc{t}, \uucstar{t} \big)\, \dt \rVert \geq \epsilon
%	\end{equation}
	holds for $\lVert \xf - \xs \rVert > 0$.
	If $\tfstar$ is finite, there also exist a scalar $\mu>0$ which satisfies $\epsilon = \mu \tfstar$
	and a suitable upper bound is given by
%\begin{equation}
$\tfstar \leq \lVert \xf - \xs \rVert/\mu = \alpha_2 \big( \lVert \xs - \xf \rVert \big).$
	%\end{equation}
	
	The previous derivation assumed $\tfstar$ to be finite and the unbounded case is now proven by contradiction.
	Consider the case in which the distance $\lVert \xf - \xs \rVert$ is unbounded.
	Now assume that $\tfstar$ is still bounded. The integral over the closed interval $[0, \tfstar]$ with bounded integrand $\f$ is bounded.
	Obviously, equality $\lVert \xf - \xs \rVert = \lVert \int_{0}^{\tfstar} \f\big(  \xc{t}, \uucstar{t} \big)\, \dt \rVert$ does not
	hold anymore which proves the claim. 
	Consequently, $\lVert \xs - \xf \rVert$ is unbounded if $\tfstar$ is unbounded and so~\eqref{eq:uniform:bounded_cost_function} is satisfied
	for the unbounded case ($\Kinffun$ rather than $\Kfun$). 	
	
	Finally, consider the case $\tfmin > 0$. Obviously, $\tfstar \geq \tfmin$ holds due to the feasibility assumption. % to \refassump{assum:uniform:optimal_solution}).
	%Consequently, for any $\xmu(\tmud{n}) \in P_{N\vardtmin}(\xf)$ the cost function does not decrease anymore can hence not be bounded from above
	By \reflem{lemma:const_cost_dtstar_dtmin}, $\xs \notin \Pfull{N}{\tfmin}$ implies $\tfstar > \tfmin$ and hence does not affect the previous results for the existence of $\alpha_1$ and $\alpha_2$.
	On the other hand, $\xmu \in \Pfull{N}{\tfmin}$ implies that $\tfstar$ is constant such that $\alpha_1$ and $\alpha_2$ do not exists.
	However, this particular case is excluded in \reflem{lemma:cost_lyapunov_bounds}.
%	\qed
\end{IEEEproof}

\begin{IEEEproof}[Proof of Theorem~\ref{shrinking_horizon_mpc:p_stability}]
	The proof relies on the Lyapunov stability theory according to Definitions~\ref{thm:lyapunov_asymp_stab} and~\ref{thm:lyapunov_p_stab}.
	Let $P$ abbreviate $P\mdef \Pxfshrinking$, $\xmu$ the current state $\xmu \mdef \xmuc{\tmud{n}}$ and $\xmu^+$ the successor state $\xmu^+ \mdef  \xmusolfun\big(\tmud{n+1},\tmud{n}, \xmu(\tmud{n}) \big)$. % \xmu(\tmud{n+1}) \mdef
	It is necessary to find a function $\fundef{V}{\rxset}{\realposzero}$ and $\alpha_1, \alpha_2\in \Kinffun, \alpha_3 \in \Kfun$ such that
	%\begin{equation}
	$\alpha_1 \big( \lVert \xmu - \xf \rVert \big) \leq V(\xmu) \leq \alpha_2 \big( \lVert \xmu - \xf \rVert \big)$ (see \eqref{app:eq:lyapunov_fun1})
%\label{eq:uniform:shrinking:lyapunov1}
	%\end{equation}
	and
	%\begin{equation}
	$V(\xmu^+) \leq V(\xmu)  - \alpha_V \big( \lVert \xmu - \xf \rVert \big)$ (see \eqref{app:eq:lyapunov_fun2})
	%\label{eq:uniform:shrinking:lyapunov2}
	%\end{equation}
	hold for all $\xmu,\xmu^+ \in \rxset\setminus P$. % with $\xmu(\tmud{n+1}) \in \rxset\setminus P$ and $n\in\naturalzero$. 

	As for \MPC{} in general, $V$ is chosen as the optimal cost function value.	
	%Since, $0 <\vardtmin < \vardtstar$ holds for the first solution at $\tmud{0}$.
	\reflemc{lemma:cost_lyapunov_bounds} ensures the first condition~\eqref{app:eq:lyapunov_fun1} for all $\xmu \notin \Pfull{N}{N\vardtmin}$.
	%However, \refthm{shrinking_horizon_mpc:p_stability} rather requires~\eqref{eq:uniform:shrinking:lyapunov1} to hold for $\xmu(\tmud{0}) \notin \Pxfshrinking$ and obviously it is $\Pxf{\Nmin} \subseteq \Pxf{N}$.
	Since \refthm{shrinking_horizon_mpc:p_stability} demands to choose $0 \leq \vardtmin < \vardtstar(\xs,N)$ for the first \OCP{}, $\tfstar(\xs,N) > N\vardtmin$ implies $\xmu \notin \Pfull{N}{N\vardtmin}$ according to \reflem{lemma:const_cost_dtstar_dtmin}.
	Consequently, condition~\eqref{app:eq:lyapunov_fun1} is satisfied regardless of $P$.
	%Consequently, condition~\eqref{eq:uniform:shrinking:lyapunov1} is satisfied for $\xmu(\tmud{0}) \notin \Pxf{\Nmin}$.
	
	Proving the second condition~\eqref{app:eq:lyapunov_fun2} follows the dynamic programming principle~\cite{bertsekas1995_book} and hence its mathematical exposition is kept brief.
	For practical stability, the Lyapunov conditions must only be ensured for $\xmu \in \rxset \setminus P$.
	The solution to the first \OCP{} at time $\tmud{0}$ is feasible by assumption and hence an admissible control trajectory $u \in \uadmset{\xs}{\tfstar(\xs,N)}$ exists. % The optimal time interval is $\vardtstar$.
	%	To emphasize its direct relation to the optimal control problem at time instance $\tmud{n}$, the optimal time interval is now denoted by $\vardtstar.
	Note that the grid is adapted with $N_0\mdef N$ and $N_{n+1} \mdef \max(N_{n} - 1,\Nmin)$.	
	First, consider the case $N_n > \Nmin$.
	The optimal cost function value is $V(\xmu) = \tfstar(\xmu, N_n)$.
	Applying the principle of optimality results in
	\begin{align}
	\tfstar(\xmu,N_n) &= \vardtstar(\xmu,N_n) + (N_n-1) \vardtstar(\xmu,N_n) \nonumber \\
	&= \vardtstar(\xmu,N_n) + (N_n-1) \vardtstar(\xmu^+,N_n-1) \nonumber \\
	\Leftrightarrow  V(\xmu) &= \vardtstar(\xmu,N_n) + V(\xmu^+).
	\label{eq:dyn_prog_time_optimal}
	\end{align}
	To ensure condition~\eqref{app:eq:lyapunov_fun2}, $\vardtstar(\xmu, N_n) \geq \alpha_V \big( \lVert \xmu - \xf \rVert \big)$ must hold for $\alpha_V \in \Kfun$.
	According to \reflem{lemma:cost_lyapunov_bounds}, $\alpha_V = \tf(\xmu,N_n)/N_n = \alpha_1 \big( \lVert \xmu - \xf \rVert \big) / N_n$ provides a suitable upper bound for $\xmu \in \rxset \setminus \Pfull{N_n}{N\vardtmin}$ % TODO: wir haben hier Pc(N_n)?? Nicht N!!!!
	and $N_n\geq\Nmin>0$ is ensured by definition. % TODO benötigt????
	As stated previously, $\xmu \notin \Pfull{N_n}{N\vardtmin}$ follows from \reflem{lemma:const_cost_dtstar_dtmin} and $\vardtstar(\xs,N_n) > \vardtmin$ as $\vardtstar(\xmu,N_n)$ remains constant for all $N_n > \Nmin$ (see~\eqref{eq:dyn_prog_time_optimal}). % TODO: letzteres vielleicht noch ausführlicher einbauen, wir droppen das hier einfach
	
	Note, the principle of optimality~\eqref{eq:dyn_prog_time_optimal} implies recursive feasibility and hence forward invariance on~$\rxset$ for $N_n > \Nmin$.
	As soon as $N=\Nmin$ is reached, control law~\eqref{eq:mulaw_adapt} performs one more step with $\vardtstar(\xs,N)$.
	Afterwards, $\vardtstar(\xmu,\Nmin)$ decreases in each step (see \reffig{fig:practical_stab_illustration}) until the lower bound $\vardtstar(\xmu,\Nmin)\geq\vardtmin$ becomes active.
	This in turn leads to a potential lack of recursive feasibility and hence forward invariance cannot be ensured in $P$ % TODO: extra lemma für forward invariance, und das P die richtige beschreibung ist?
	which limits the stability results to $\rxset \setminus P$.	
	%\qed
\end{IEEEproof}
